# Supplementary material for: Security Vetting Process of Smart-home Assistant Applications: A First Look and Case Studies
Source: arXiv:2001.04520 source file (2020-01-13)
Supplement: Supplementary file 1 [file appendix.tex]

\section*{Appendix - Ethical Considerations}
Below, we provide a more detailed discussion regarding the ethical aspects and considerations for our experiments.

\para{A: Proof-of-Concept Attacks.}
Throughout the experiments, both the attacker endpoint and the victim endpoint are developed by ourselves. The tests are conducted in the developer mode. There are no other skill endpoints or users involved in this experiment. 

\para{B: Publishing a Vulnerable Skill.} We took active steps to ensure research ethics. At the high level, this skill is a ``vulnerable'' skill instead of a ``malicious'' skill. It is supposed to be the victim instead of the attacker in the threat model, which should not introduce any malicious impact. There are still a number of considerations and actions we take to protect users. First, one concern of publishing a vulnerable skill is that the skill may be accidentally used by an innocent user. To avoid this, we have closely monitored our skill endpoint throughout the releasing process. Once the skill received the approval, we immediately performed a quick test to ensure the skill is truly available on the store, and then took it down from the store right away. During this process, we monitored our server and we did not see any incoming requests (except those from our own). This means no real users have ever used this vulnerable skill. Second, the released skill is about providing information, without collecting any user data. Even if a user accidentally used the skill, there is no actual harm. Third, after the experiment, we immediately contacted Google and Alexa team to inform them about our research and offer our help to improve the current system. 

\para{C: Network Scanning.}
We perform network scanning to locate vulnerable skill endpoints.
First, for each host, we only send a handful of queries which has minimal impact of the target host. Second, we re-use the ZMap scanning results~\cite{zmap13} instead of performing our own network-wise scanning to locate live HTTPS hots. Our scanning scope is also aligned with ZMap port 443 scanning. We respect Internet hosts that don't want to be scanned by ZMap and did not test these hosts. Third, we only test non-intrusive Intent that does not cause any internal state change of the skill service or reveal any non-public information. The query carries the spoofed ``LaunchRequest'' intent which is a default intent that every Alexa skill should support. ``LaunchRequest'' should only trigger a welcoming message.
